# Supplementary material for: Bootstrap an end-to-end ASR system by multilingual training, transfer learning, text-to-text mapping and synthetic audio
Source: arXiv:2011.12696 source file (2021-06-18)
Supplement: Supplementary file 1 [file appendix.tex]

\subsection{More details about ASR model training}

The WarmHoldDecayLRScheduler is used for learning rate scheduling in
the training of all models.
The multilingual training approach adopts the following learning-rate strategy:
For the first 4,000 steps, learning rate increased from 1e-7 up to 5e-4.
A second phase continued until step 140,000, where learning rate was kept constant.
Finally, the last phase of exponential decay brought learning rate down to 1e-5 until step 280,000.
For the transfer learning, we used the following learning rate strategy:
For the first 2,000 steps, learning rate increased from 1e-7 up to 5e-4.
A second phase continued until step 20,000, where learning rate was kept constant.
Finally, the last phase of exponential decay brought learning rate down to 1e-5 until step 35,000.
For all models we trained, the work was distributed across 3 hosts, with 8 GPUs each.
Batch size was set to 64 for utterances shorter than 300 frames.

\subsection{Comparison with production hybrid models}
\label{sec:compare_with_production_asr}

Here we provide a comparison of the models mentioned in this work with the
real it-IT models that are currently in Production or were used in 2018 as beta models.
Note that the training and evaluation data used are different so the numbers should
not be compared strictly, still Table \ref{tab:tts_on_low_resource_extended}
provides a glance over accuracy range of ASR boostrapped in this work and
ASR built in traditional approaches.

\begin{table}[th]
  \caption{Same experiment setup as Table \ref{tab:tts_on_low_resource}, but also including the prod hybrid models as comparison.}
  \label{tab:tts_on_low_resource_extended}
  \centering
  \begin{tabular}{ l l l l c }
    \toprule
    \textbf{Model} & \textbf{RNN-T} & \textbf{Transfer} & \multirow{2}{*}{\textbf{Translation}} & \textbf{SER} \\ % \textbf{SA} \\
    \textbf{index} & \textbf{seed}  &  \textbf{learning} &  & (\%) \\
    \toprule
    1 & M & - & - & 70.5 \\			% 29.5 \\
    \midrule
    2 & M & - & TTS & 66.9 \\ 			% 33.1 \\
    3 & M + TTS & - & - & 66.2 \\ 		% 33.8 \\
    \midrule
    4 & M & - & R + TTS & 52.8 \\ 		% 47.2 \\
    5 & R & - & - & 38.0 \\ 			% 62.0 \\
    6 & M + R & R & - & 30.4 \\ 		% 69.6 \\
    7 & M + R & R & R + TTS & 28.3 \\ 		% 71.7 \\
    8 & M + R & R + TTS & -  & 25.5 \\ 		% 74.5 \\
    9 & M + R & R + TTS & R + TTS & 24.7 \\ 	% 75.3 \\
    \midrule
    R1 & \multicolumn{3}{l}{it-IT v2 (beta entry model)} & 52.3 \\ 	% 47.7 \\
    R2 & \multicolumn{3}{l}{it-IT v13 (GA launch model)} & 26.3 \\ 	% 73.7 \\
    R3 & \multicolumn{3}{l}{it-IT v32 (current prod model)} & 15.0 \\ 	% 85.0 \\
    \midrule
    \bottomrule
  \end{tabular}
\end{table}

In terms of the number of hours of audio available:
the beta-entry model was trained with approximately 200 hours of audio,
the GA launch model was trained with approximately 600 hours of audio,
and the production model was trained with approximately 10,000 hours of audio.

\subsection{Future work by milestones}

\begin{itemize}
    \item \textbf{M1} (3 weeks): ICASSP 2021 submission.
    \item \textbf{M2} (8 weeks): Bootstrap an Arabic RNN-T model using multilingual 
    	transfer learning, TTS and post-ASR translation/error-correction,
	in combination with available non-Alexa Arabic data for ASR bootstrapping.
    \item \textbf{M3} (6 weeks): Switch to word-piece based translation for Arabic,
	and investigate the benefit of using advanced neural machine translation
	models. In addition, investigate using phoneme-level output to support the
	translation model.
    \item \textbf{M4} (6 weeks): Use teacher student training to combine and
	transfer knowledge between different ASR architectures, i.e. the bootstrapped
	Arabic ASR based on RNN-T and translation model, and the standard Arabic
	hybrid ASR being developed in a parallel thread.
\end{itemize}

\subsection{Future work per tech aspect in details}

\textit{Better TTS:}
The bootstrapping results with TTS were underwhelming, especially
in the zero-data case.
This is partly due to the acoustic mismatch between synthetic speech and real 
speech that originates in the design of TTS.
Future work will explore more advanced TTS 
with more voices and speaking styles, to validate whether the acoustic mismatch
could be reduced. In addition, techniques like encoder freezing could
be explored as to alternatively mitigate the risk in acoustic mismatch
when an better TTS is not available.

\textit{All-neural translation:}
In this work we choose to work with an FST-based translation algorithm,
mainly due to the need for rapid and inexpensive experimentation.
A logical next step is to use a more expensive and powerful seq2seq model.

\textit{Bootstrapping with out-of-domain-data:}
In the experiments, we investigated how to optimally use a minimal amount of TTS and production data.
A different direction of work is to ensure that out-of-domain datasets available (like Amazon Prime Video)
could be used effectively to bootstrap Alexa in a new language. 
One challenge we foresee already is the mismatch in acoustic conditions and 
vocabulary.

\textit{Using worpieces for translation:}
The current translation system focused on word-level translation. This makes sense, as our multilingual model
was trained on Romance languages, and our target was Italian. 
On the other side, languages like Arabic are very different,
using smaller wordpieces or phones might have more potential in bootstrapping
distant languages.

\textit{Smooth exit from bootstrapping phase:}
The strategy investigated in this work has a big potential during early bootstrapping
phase, but it needs a smooth transition to language specific RNN-T 
as the amount of available training data builds up in target language and target
domains. Such transition is critical in real application. One option is 
knowledge distillation via teacher student training, where teacher ASR is the
bootstrapping system with translation based error correction, and this method
could be combined with training on unsupervised data. Another option is
to keep ensembles of ASR systems and integrate the recognition output via
confidence based voting. This allows the bootstrapping system to lead when
the locale specific ASR model builds up over time, followed by a natural and 
smooth overtake from the locale specific ASR model once it is ready.

\textit{Arabic ASR:}
Techniques investigated in this work can be validated in a production setup 
to speed up the ongoing ASR bootsrapping for Arabic Alexa.
In particular, synthetic Arabic data from Polly TTS can be added to ASR training,
and to the error correction model optimization for Arabic ASR in early development.
In addition, teacher student training could explored to transfer knowledge across
ASR model architecture. Finally, experimenting with Arabic allows investigation on challenges in language with multiple written scripts.
